# Supplementary material for: Large spin-mixing conductance in highly Bi-doped Cu thin films
Source: arXiv:1806.01394 source file (2018-07-24)
Supplement: Supplementary file 1 [file SRuizGomez_SuppInfo.pdf]

**Supporting information:**

# Highly Bi-doped Cu thin films with large spin-mixing conductance

Sandra Ruiz-Gómez,[1] Aída Serrano,[2] Rubén Guerrero,[3] Manuel Muñoz,[4] Irene Lucas,[5,6] Michael Foerster,[7] Lucia Aballe,[7] José F. Marco,[8,9] Mario Amado,[10] Lauren McKenzie-Sell,[10] Angelo di Bernardo,[10] Jason W. A. Robinson,[10] Miguel Ángel González Barrio,[1,9] Arantzazu Mascaraque,[1,9] and Lucas Pérez[1,3,9]

[1]) *Dept. Física de Materiales. Universidad Complutense de Madrid. 28040 Madrid, Spain*

[2]) *SpLine, Spanish CRG BM25 Beamline, ESRF, 38000 Grenoble, France*

[3]) *Instituto Madrileño de Estudios Avanzados - IMDEA Nanociencia, 28049, Madrid, Spain*

[4]) *Instituto de Micro y Nanotecnología (CNM-CSIC), PTM, 28760 Tres Cantos, Madrid, Spain*

[5]) *Dpto. Física de la Materia Condensada, Universidad de Zaragoza, Pedro Cerbuna 12, 50009 Zaragoza, Spain*

[6]) *Instituto de Nanociencia de Aragón (INA), Universidad de Zaragoza, Mariano Esquillor, Edificio I+D, 50018 Zaragoza, Spain*

[7]) *Alba Synchrotron Light Facility, CELLS, E-08290, Carrer de la Llum 2-23, Bellaterra, Spain*

[8]) *Instituto de Química Física Rocasolano - CSIC, Calle de Serrano, 119, 28006 Madrid, Spain*

[9]) *Unidad Asociada IQFR (CSIC)-UCM, 28040, Madrid, Spain*

[10]) *Department of Materials Science and Metallurgy, University of Cambridge, 27 Charles Babbage Road, Cambridge CB3 0FS*

## I. GROWTH OF THE YIG SUBSTRATES

Lattice match 110-oriented comercial gadolinium gallium oxide substrates were pre-cleaned rinsed sequentially with DI water, acetone and isopropyl alcohol and annealed ex-situ under a 100 sccm constant flow of oxygen at 1000°C for 8 hours with a ramping rate of 10°C/min. The substrates were then placed in a pulse laser deposition (PLD) chamber with a base pressure of $5 \times 10^{-7}$ mbar. YIG thin films were deposited by PLD using a KrF 248-nm wavelength excimer laser. The films were grown under a stable atmosphere of 0.1 mbar of $O_2$ at 750°C. The KrF excimer laser pulses had a power of 450 mJ (and a fluence of 2.2 $W/cm^2$) and strike a polycristalline target of YIG for 21600 pulses at a constant frequency of 4Hz. An in-situ post-annealing at 850°C was performed for 2 hours under a 0.5 mbar static environment of ultra-pure $O_2$ and subsequently cooled down to room temperature at -10°C/min.

## II. X-RAY PHOTOELECTRON SPECTROSCOPY

Figure S.1 collects the wide scan spectra recorded at different sputtering times from a $Bi_{85}Cu_{15}$ thin film. For the figure it can be seen that the spectrum of the as-grown sample show only XPS signals coming from Cu, Bi, O and C. As the sputtering time increases, the intensity of the C and O signals decreases strongly while the Cu 2p peaks increases, which can be linked to the removal of the contamination layer from the uppermost surface. The C and O signals are really small after long sput tering times. The spectra also show a clear increase of the intensity of the Cu 2p peaks with increasing sputter ing time. However, more than due to an increase in Cu concentration this must be related, as explained in the manuscript, to a much smaller, almost insignificant, attenuation of the Cu 2p electrons once the contamination layer has been removed from the uppermost surface compared to the attenuation of the Bi electrons.

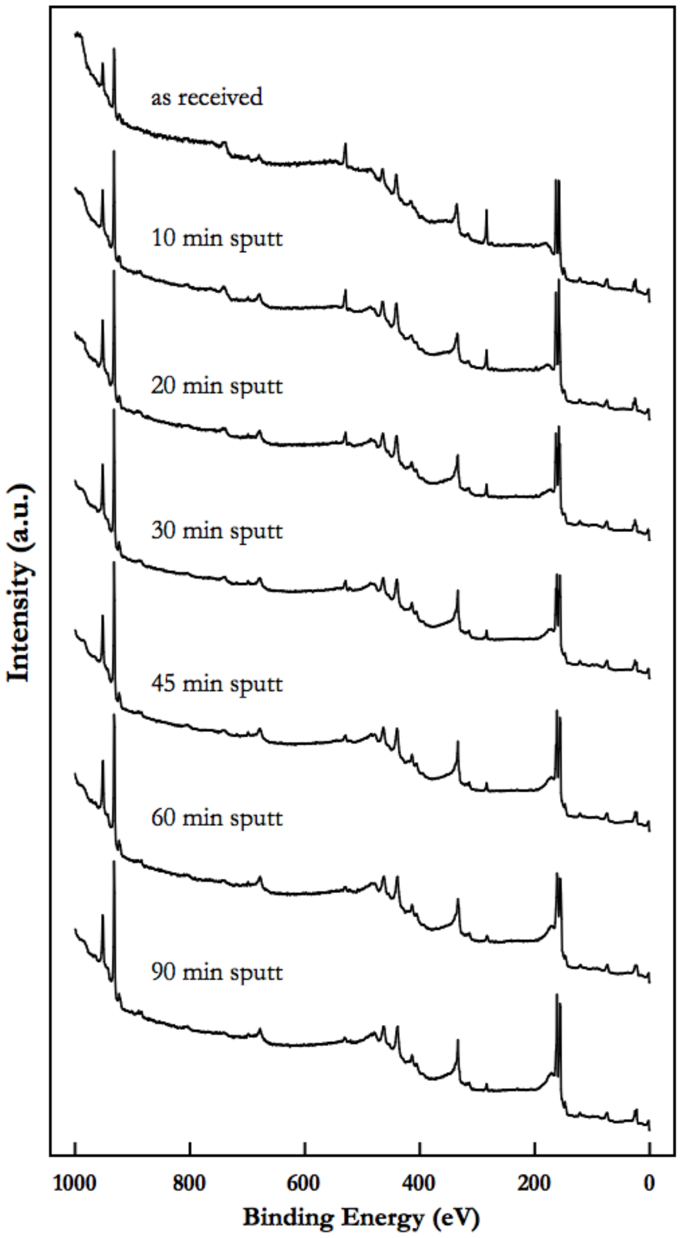


FIG. S.1. XPS wide scan spectra recorded from the $Bi_{15}Cu_{85}$ sample at different sputtering times.

## III. FERROMAGNETIC RESONANCE MEASUREMENTS

Figure S.2 shows FMR measurements at RT carried out in two CuBi/YIG samples with different Bi concentration. The FMR was measured using the the configuration mentioned in the experimental section, where the dP/dH was recorded as a function of constant applied DC magnetic field. The FMR linewidth was taken as the difference of fields between the maximum and minimum of the dP/dH curve and the resonance field was determined as the

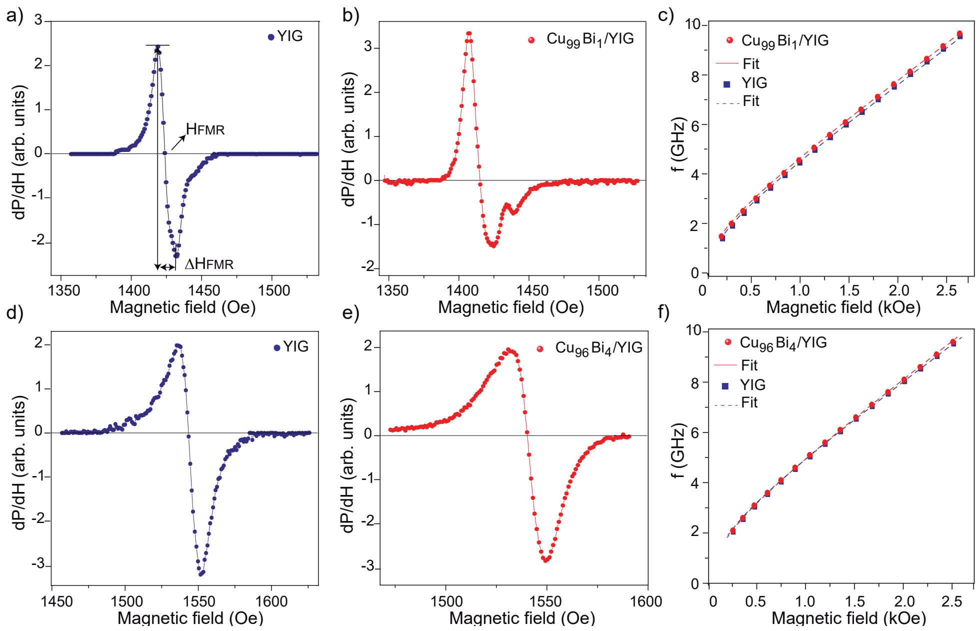


FIG. S.2. Dependence on dP/dH curve of applied DC magnetic field for sample $Cu_{99}Bi_1$ at 6 GHz before (a) and after (b) CuBi deposition. (c) Dependence of resonant field on frequency for the previous sample. (d) and (e) Dependence on dP/dH curve of applied DC magnetic field for sample $Cu_{96}Bi_4$ at 6 GHz before and after CuBi deposition, respectively. (f) Dependence of resonant field on frequency for the previous sample.

intersection of the dP/dH curve, with zero (Figure S.2.a). Figure S.2c. and Figure S.2 f. shows a typical curve of resonance frequency vs DC magnetic field for CuBi/YIG before and after CuBi growth. The continuous line corresponds to the fitting of experimental data using Kittel's equation.
